# Supplementary material for: Nodeless Hybridization as Proof of Trivial Topology in Samarium Hexaboride
Source: arXiv:2505.06449 ancillary file (2025-05-09)
Supplement: Supplementary file 1 [file Supplementary_Material.pdf]

# Supplementary Material
# Nodeless Hybridization as Proof of Trivial Topology in Samarium Hexaboride

E. D. L. Rienks[1,§] P. Hlawenka[1] J. Sánchez-Barriga[1,2]
E. Schierle[1] M. Jugovac[3] P. Perna[2] Kai Chen[1,+]
K. Siemensmeyer[1] E. Weschke[1] A. Varykhalov[1]
N. Y. Shitsevalova[4] V. B. Filipov,[4] S. Gabáni[5]
K. Flachbart[5] O. Rader[1,*]

May 9, 2025

## Supplementary Note 1: Dimensionality of the conduction band photoemission intensity at $\bar{X}$

At 50 K, the conduction band is partially thermally occupied and can be observed, as reported previously (*1*, *2*). In Fig. S1(a-e), we show photoemission spectra at 50 K for perpendicular momenta of $3.8\pi/a$ to $4.2\pi/a$ (photon energies from 23 to 31 eV) in the vicinity of $\bar{X}$. The topmost spectra are measured at $\bar{X}$ and the sequence below are for $k_{||}$ in the direction towards $\bar{\Gamma}$. It is seen that the conduction band is observed at $\bar{X}$ only in a narrow momentum range with a peak exactly at $4.0\pi/a$. In Fig. S1(g) the ratio of conduction band and valence band intensities is displayed following a decomposition as shown for 27 eV in Fig. S1(f). The next appearance of the conduction band is at $6.0\pi/a$, seen in Fig. S1(h) around 70 eV photon energy. Fig. S1(i) shows that the conduction band lies inside of the elliptical constant energy contours probed here.

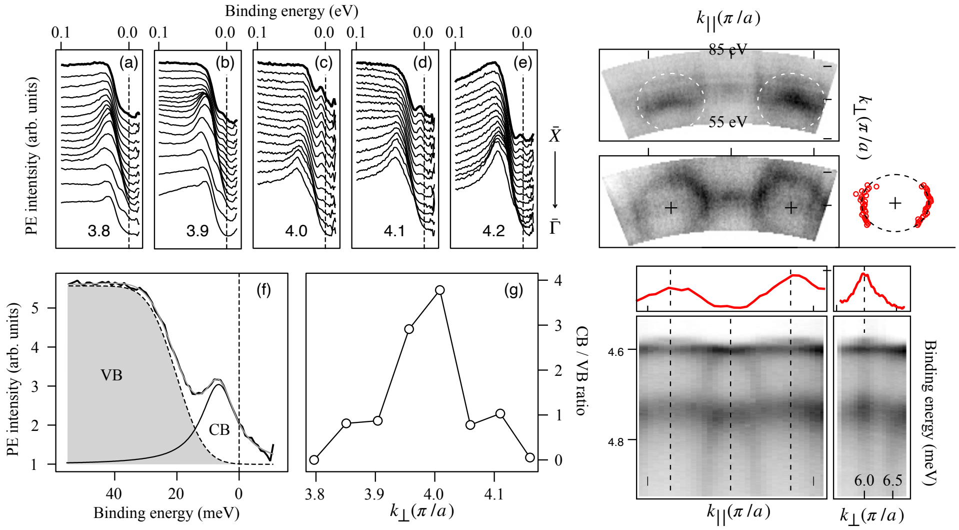


Figure S 1: The conduction band appears at $\bar{X}$ only for photon energies corresponding to $k_\perp = 2n\pi$. (a–e) Energy distribution curves along the $\bar{X}$– $\bar{\Gamma}$ direction for photon energies between 23 and 31 eV at $T = 50$ K. (f) Relative intensities of the valence and conduction bands are determined by fitting with a superposition of a step function (VB) and a Lorentzian component (CB). (g) Intensity ratio of the conduction and valence band at $\bar{X}$ as a function of $k_\perp$. (h,i) Alternative probe of the conduction band near 70 eV. (h) Conduction band probed near $E_\mathrm{F}$ and (i) bulk $5d$ states.

# Supplementary Note 2: Limitations by momentum resolution

Given the very weak dispersion of the predominantly $f$-like section of the conduction band near $X$, it is tempting to immediately conclude that the experimentally observed shift reflects a shift of the 3-D band structure at $X$. We have, however, to assess whether an imperfect $k_\perp$ resolution could suggest a shift at $X$ that actually takes place away from $X$. We have seen above (Fig. 1) that the unmixed $f$ state must disperse at least weakly such that $\varepsilon_f(X)$ lies above $\varepsilon_f(\Gamma)$. Consequently, the conduction band formed by relatively weak mixing will have a 'W'-like profile, see Fig. 1. Increasing the hybridization ($V$) gives rise to a more 'U'-like shape, while the dispersion at $X$ remains pinned at the unmixed position.

Let us assume that $k_\perp$ resolution in the ARPES experiment is insufficient to resolve the dispersion of the 3-D conduction band along the out-of-plane direction ($\Gamma$-$M$ in this orientation). The observed photoemission maximum is then due to the integrated spectral weight of the entire $f$-like section of the conduction band. For smaller $V$ (i.e., at higher $T$) inclusion of the higher binding energy valleys away from $X$ will give rise to a larger apparent binding energy in the experiment compared to the more strongly hybridized (U-like, lower $T$) case. Can this effect account for the experimentally observed shift of the conduction band with $T$?

We will examine the plausibility of this scenario by means of a simple simulation: We estimate the $f$ and $d$ dispersion based on earlier work: The three $4f$ states comprising the $\mathrm{SmB_6}$ valence structure are, in the topological Kondo insulator scenario, degenerate at Γ, see Fig. 3 of Lu *et al.* (*4*), with a binding energy of 15 meV (see Fig. 2 in the main text and Hlawenka *et al.* (*5*)). For the conduction band to be entirely unpopulated in the ground state, the dispersion must lie more than $5$ meV above the Fermi energy at $X$. The itinerant $5d$ state has a maximum binding energy of $1.7$ eV at $X$ and a band width to yield an electron pocket of the appropriate Fermi wave vector $k_\mathrm{F}$. This has the following consequences:

First, the maximal shift we can expect is limited by the $f$ dispersion and is still smaller than the observed shift by a factor of 3–5.

Second, the weakly mixed (i.e., high temperature) conduction band has, as a result of the $k_\perp$-integrated W-profile, a plano-convex intensity profile with a flat bottom. In contrast, the experimentally observed conduction band is at all temperatures found to have a U-shape. Note that this U-shape must not be confused with the U-shape in Fig. 1. The present U crosses the Fermi level whereas the U in Fig. 1 is fixed above the Fermi level due to the topological Kondo insulator

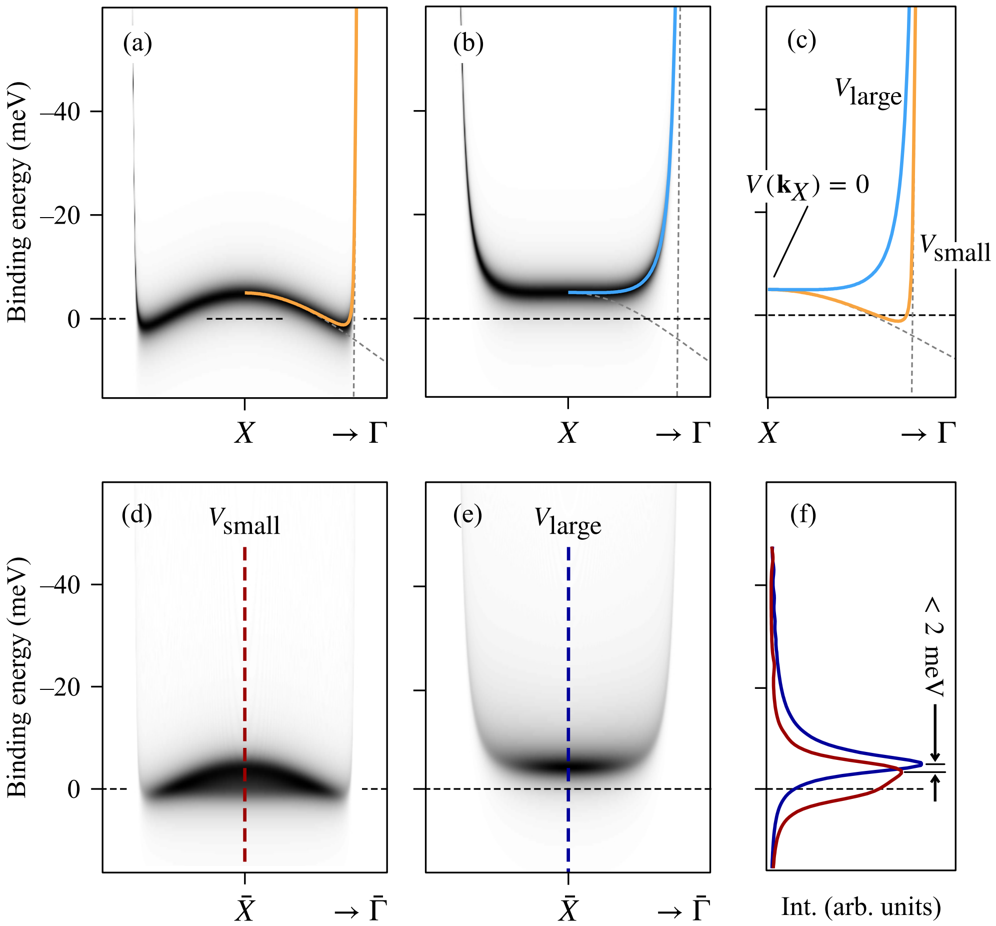


Figure S 2: Simulation of finite momentum resolution. (a) In a topological Kondo insulator (*3*) a gap opens by hybridization between bands for $\mathbf{k}$ values between high-symmetry points.

scenario and is unlikely to become occupied even at the highest temperatures.

Third, the photon energy dependent ARPES measurements in Fig. S1 show that the $k_\perp$ resolution is fairly good: We do not observe smearing of the conduction band intensity beyond the envelope provided by the $5d$ band dispersion.

# References


*1.* C.-H. Min *et al.*, *Phys. Rev. Lett.* **112**, 226402 (2014).

*2.* J. D. Denlinger *et al.*, arXiv: `1312.6637v1 (cond-mat.str-el)` (2013).

*3.* M. Dzero, J. Xia, V. Galitski, P. Coleman, *Annu. Rev. Condens. Matter Phys.* **7**, 249–280 (2016).

*4.* F. Lu, J. Zhao, H. Weng, Z. Fang, X. Dai, *Phys. Rev. Lett.* **110**, 096401 (2013).

*5.* P. Hlawenka *et al.*, *Nat. Commun.* **9**, 517 (2018).
